# Supplementary material for: Differential Privacy Dynamics of Langevin Diffusion and Noisy Gradient Descent
Source: arXiv:2102.05855 source file (2022-09-09)
Supplement: Supplementary file 1 [file appendix_main.tex]

% !TEX root = ../main.tex

% \section{Appendix}
% \label{sec:appendix}

 \input{appendices/symbol_table}
 \input{appendices/calculus_refresher}
 \section{Proofs for privacy analysis of Langevin Diffusion}
\label{sec:diffusion_proof}

\begin{replemma}{lem:marginalrenyi}[ Rate of R\'enyi Privacy Loss ]
Let $\loss{\x}{\ptheta}$ be a loss function on $\thetaspace$, with a finite total gradient sensitivity $\sen{\g}$. Then for coupled Langevin diffusions $\{\thet_t\}_{t\geq0}$ and $\{\thet_t'\}_{t\geq0}$ on neighboring datasets $\D, \D' \in \Domain$, under loss ${\smaloss{\x}{\ptheta}}$ and noise variance $\tnoise^2$, the R\'enyi privacy loss rate at any $t\geq0$ is upper bounded by
\begin{equation}
    \doh{\Ren{\q}{\thet_{t}}{\thet_{t}'}}{t}
    \leq 
    \frac{1}{\gamma}\frac{\q S_g^2}{4\tnoise^2\size^2}
    -
    (1-\gamma)\tnoise^2\q \frac{\Gren{\q}{\thet_{t}}{\thet_{t}'}}{\Fren{\q}{\thet_{t}}{\thet_{t}'}}.
\end{equation}
where $\gamma>0$ is a tuning parameter that we can fix arbitrarily according to our need.
\end{replemma}

\begin{proof}
    For brevity, let the functions ${R(\q,t)=\Ren{\q}{\rhO_{t}}{\rhO_{t}'}}$, ${E(\q,t)=\Fren{\q}{\rhO_{t}}{\rhO_{t}'}}$, and ${I(\q,t)=\Gren{\q}{\rhO_{t}}{\rhO_{t}'}}$. Under the stated assumptions $\doh{E(\q,t)}{t}$ is bounded as follows.
    \begin{align*}
        \doh{E(\q,t)}{t} &=\doh{}{t}\int_{\thetaspace}\frac{\rhO_{t}^{\q}}{\rhO_{t}'^{\q-1}}\dif{\ptheta} \\
        &= \q \int_{\thetaspace} \doh{\rhO_{t}}{t} \left(\frac{\rhO_{t}}{\rhO_{t}'}\right)^{\q-1}\dif{\ptheta} \\
        &\quad    -(\q-1) \int_{\thetaspace} \doh{\rhO_{t}'}{t} \left(\frac{\rhO_{t}}{\rhO_{t}'}\right)^{\q} \dif{\ptheta} \\
        &=\ \q\int_{\thetaspace} \left(\tnoise^2\lapL{\rhO_{t}} + \divR{(\rhO_{t}\graD{\Loss(\D)})}\right)
            \left(\frac{\rhO_{t}}{\rhO_{t}'}\right)^{\q-1}\dif{\ptheta} \\
        &\quad -(\q-1)\int_{\thetaspace} \big(\tnoise^2\lapL{\rhO_{t}'}+ \divR{(\rhO_{t}'\graD{\Loss(\D')})}\big) \\
        & \quad\quad\quad\quad\quad\quad\quad\quad\quad
            \left(\frac{\rhO_{t}}{\rhO_{t}'}\right)^\q\dif{\ptheta}
            \tag{From \eqr{eqn:fokkerplanck}} \\
        &   \begin{rcases}
                =\tnoise^2 \q\int_{\thetaspace}\left(\frac{\rhO_{t}}{\rhO_{t}'}\right)^{\q-1}\lapL{\rhO_{t}}\dif{\ptheta} \\
                \quad -\tnoise^2(\q-1)\int_{\thetaspace}\left(\frac{\rhO_{t}}{\rhO_{t}'}\right)^{\q}\lapL{\rhO_{t}'}\dif{\ptheta}
            \end{rcases} \eqdef F_1 \\
        &   \begin{rcases}  
                \quad +\q\int_{\thetaspace}\left(\frac{\rhO_{t}}{\rhO_{t}'}\right)^{\q-1} \divR{(\rhO_{t}\graD{\Loss(\D)})}\dif{\ptheta} \\
                \quad -(\q-1)\int_{\thetaspace}\left(\frac{\rhO_{t}}{\rhO_{t}'}\right)^{\q} \divR{(\rhO_{t}'\graD{\Loss(\D')})}\dif{\ptheta}
            \end{rcases} \eqdef F_2
    \end{align*}
    Now $F_1$ is equivalent to the following.
    \begin{align*}
        F_1 &= \tnoise^2(\q-1)\int_{\thetaspace}\dotP{\graD{\left(\frac{\rhO_{t}}{\rhO_{t}'}\right)^\q}}{\graD{\rhO_{t}'}}\dif{\ptheta} \\
            &\quad -\tnoise^2 \q\int_{\thetaspace}\dotP{\graD{\left(\frac{\rhO_{t}}{\rhO_{t}'}\right)^{\q-1}}}{\graD{\rhO_{t}}}\dif{\ptheta}
                \tag{From \eqr{eqn:lapl_dotp_eq}} \\
            &= \tnoise^2 \q(\q-1)\int_{\thetaspace} \negthickspace\left(\frac{\rhO_{t}}{\rhO_{t}'}\right)^{\q-2}\negthickspace\negthickspace\dotP{\negthickspace\graD{\frac{\rhO_{t}}{\rhO_{t}'}}}
                {\frac{\rhO_{t}}{\rhO_{t}'^2}\graD{\rhO_{t}'} - \frac{\graD{\rhO_{t}}}{\rhO_{t}'}\negthickspace}\rhO_{t}'\dif{\ptheta} \\
            &= -\tnoise^2 \q(\q-1)\Expec{\rhO_{t}'}{\left(\frac{\rhO_{t}}{\rhO_{t}'}\right)^{\q-2} \norm{\graD{\frac{\rhO_{t}}{\rhO_{t}'}}}^2}
                \tag{$\because \graD{\frac{\rhO_{t}}{\rhO_{t}'}} = \frac{\graD{\rhO_{t}}}{\rhO_{t}'} - \frac{\rhO_{t}}{\rhO_{t}'^2}\graD{\rhO_{t}'}$} \\
            &= -\tnoise^2 \q(\q-1) I(\q, t) \tag{From \eqr{eqn:grenyi_divergence}}
    \end{align*}
    And $F_2$ is upper bounded by the following.
    \begin{align*}
        F_2 &= (\q-1)\int_{\thetaspace}\dotP{\graD{\left(\frac{\rhO_{t}}{\rhO_{t}'}\right)^{\q}}}{\rhO_{t}' \graD{\Loss(\D')}}\dif{\ptheta} \\
            &\quad -\q\int_{\thetaspace}\dotP{\graD{\left(\frac{\rhO_{t}}{\rhO_{t}'}\right)^{\q-1}}}{\rhO_{t}\graD{\Loss(\D)}}\dif{\ptheta}
                \tag{From \eqr{eqn:divr_dotp_eq}} \\
            &= \q(\q-1)\negthickspace\int_{\thetaspace}\negthickspace\left(\frac{\rhO_{t}}{\rhO_{t}'}\right)^{\q-2}\negthickspace\negthickspace\dotP{\negthickspace\graD{\frac{\rhO_{t}}{\rhO_{t}'}}}
                {\frac{\rhO_{t}}{\rhO_{t}'}\graD{\left(\Loss(D') - \Loss(D)}\right)\negthickspace}\rhO_{t}'\dif{\ptheta} \\
            &\leq \gamma \q(\q-1)\tnoise^2\int_{\thetaspace}\left(\frac{\rhO_{t}}{\rhO_{t}'}\right)^{\q-2}\norm{\graD{\frac{\rhO_{t}}{\rhO_{t}'}}}^2\rhO_{t}'\dif{\ptheta}
                \tag{From \eqr{eqn:young_ineq} with $b=2\gamma\tnoise^2$} \\
            &\quad + \frac{\q(\q-1)}{4\gamma\tnoise^2}\left(\frac{S_g}{\size}\right)^2\int_{\thetaspace}\left(\frac{\rhO_{t}}{\rhO_{t}'}\right)^{\q-2}\norm{\frac{\rhO_{t}}{\rhO_{t}'}}^2\rhO_{t}'\dif{\ptheta}
                \tag{$\because {\vert\vert\graD{\smaloss{\x}{\ptheta}}-\graD{\smaloss{\x'}{\ptheta}}\vert\vert_2\leq S_g}$ by definition} \\
            &\leq \gamma\tnoise^2 \q(\q-1) I(\q,t) + \frac{1}{\gamma}\frac{\q(\q-1)S_g^2}{4\tnoise^2\size^2} E(\q,t) \tag{From \eqr{eqn:frenyi_divergence} \& \eqr{eqn:grenyi_divergence}}
    \end{align*}
    Therefore, we get the following bound on the rate of Renyi divergence.
    \begin{align*}
        \doh{R(\q,t)}{t}&=\frac{1}{\q-1}\times \frac{1}{E(\q,t)}\times\doh{E(\q,t)}{t}\\
                                                &\leq -(1-\gamma)\tnoise^2 \q\frac{I(\q,t)}{E(\q,t)} + \frac{1}{\gamma}\frac{\q S_g^2}{4\tnoise^2\size^2} 
    \end{align*}
\end{proof}

\begin{replemma}{lem:RDinLSI}[ $\alp$-LSI in terms of Rényi Divergence~\cite{vempala2019rapid} ]
    Suppose $\rhO,\rhO'$ are probability distributions of random variables $\thet_t, \thet_t'$ on $\thetaspace$. If $\frac{\rhO}{\rhO'}\in\Ftheta{\thet_t'}$, 
    then for any $\q \geq 1$, 
    \begin{align*} 
        \Ren{\q}{\thet_t}{\thet_t'} 
        + 
        \q(\q - 1) \doh{\Ren{\q}{\thet_t}{\thet_t'}}{\q}  
        \leq 
        \frac{\q^2}{2\alp} \frac{\Gren{\q}{\thet_t}{\thet_t'}}{\Fren{\q}{\thet_t}{\thet_t'}},
    \end{align*}
    if and only if $\rhO'$ satisfies $\alp$-LSI.
\end{replemma}

\begin{proof}
    For brevity, let the functions ${R(\q)=\Ren{\q}{\thet_t}{\thet_t'}}$, ${E(\q)=\Fren{\q}{\thet_t}{\thet_t'}}$, and ${I(\q)=\Gren{\q}{\thet_t}{\thet_t'}}$. 
    Let function ${g^2(\ptheta)=\left(\frac{\rhO(\ptheta)}{\rhO'(\ptheta)}\right)^\q}$. Then,
    \begin{align*}
        \Expec{\rhO'}{g^2} = \Expec{\rhO'}{\left(\frac{\rhO}{\rhO'}\right)^{\q}} = \Frenyi{\q}{\rhO}{\rhO'},
        \tag{From \eqr{eqn:frenyi_divergence}}
    \end{align*}
    and,
    \begin{align*}
        \Expec{\rhO'}{g^2 \log g^2} &= \Expec{\rhO'}{\left(\frac{\rhO}{\rhO'}\right)^{\q} 
                                   \log \left(\frac{\rhO}{\rhO'}\right)^{\q}} \\
                                   &= \q \doh{}{\q}\Expec{\rhO'}{\int_{\q}\left(\frac{\rhO}{\rhO'}\right)^{\q} 
                                   \log\left(\frac{\rhO}{\rhO'}\right)\dif{\q}}
                                   \tag{Lebniz's rule} \\
                                   &= \q \doh{}{\q}\Expec{\rhO'}{\left(\frac{\rhO}{\rhO'}\right)^{\q}}
                                   = \q \doh{E(\q)}{\q}
                                   \tag{From \eqr{eqn:frenyi_divergence}}
    \end{align*}
    Moreover,
    \begin{align*}
        \Expec{\rhO'}{\norm{\graD{g}}^2} = \Expec{\rhO'}{\norm{\graD{
        \left(\frac{\rhO}{\rhO'}\right)^\frac{\q}{2}}}^2}
        = \frac{\q^2}{4} I(\q)
        \tag{From \eqr{eqn:grenyi_divergence}}
    \end{align*}
    Substituting \eqr{eqn:lsi_standard} with the above equalities give
    \begin{align*}
            &\Ent{\rhO'}{g^2} \leq \frac{2}{\alp} \Expec{\rhO'}{\norm{\graD{g}}^2} \\
        \iff&\q\doh{E(\q)}{\q} - E(\q) \log E(\q)
            \leq \frac{\q^2}{2\alp} I(\q) \\
        \iff&\q\doh{\log E(\q)}{\q} - \log E(\q) 
            \leq \frac{\q^2}{2\alp} \frac{I(\q)}{E(\q)} \\
        \iff&\q\doh{}{\q}\left((\q-1) R(\q)\right) - (\q - 1)R(\q)
            \leq \frac{\q^2}{2\alp} \frac{I(\q)}{E(\q)}
            \tag{From \eqr{eqn:renyi_divergence}} \\
	\iff& R(\q) + \q(\q-1)\doh{R(\q)}{\q}
            \leq \frac{\q^2}{2\alp} \frac{I(\q)}{E(\q)}
    \end{align*}
\end{proof}

\begin{reptheorem}{thm:linearRDP}
	Let $\loss{\x}{\ptheta}$ be a loss function on $\thetaspace$, with a finite total gradient sensitivity $\sen{\g}$, then the Langevin diffusion under loss $\ell(\theta;\x)$ and noise variance $\sig^2$ for time $T$ satisfies $(\alpha,\eps)$-RDP for $\eps=\frac{\alpha S_g^2 T}{4\sig^2\size^2}$.
\end{reptheorem}
\begin{proof}
    Setting $\gamma=1$ in Lemma~\ref{lem:marginalrenyi} gives constant privacy loss rate. Integrating over $t$ suffices.
\end{proof}

\begin{theorem}[RDP for Langevin Diffusion under $\alp$-LSI]
    \label{thm:RDboundCD}
    For a given dataset $\database \in \Domain$ and any $t>0$, let $\{\thet_t\}_{t\geq 0}$ be the Langevin diffusion on $\database$ for loss function ${\smaloss{\x}{\ptheta}}$ and variance~$\sig^2$.  If the distribution of $\thet_{t}$ satisfies $\alp$-LSI, for any~$\database$ and any $0\leq t\leq T$, the algorithm corresponding to the Langevin diffusion satisfies $(\q,\eps)$-RDP for
    \begin{equation} 
        \eps = \frac{\q S_g^2}{2 \alp n^2 \sig^4}(1-e^{-\sig^2\alp T})
    \end{equation}
    where $\sen{\g}$ is the finite sensitivity of total gradient ${\g(\ptheta; \D) = \sum_{\x \in \D} \graD{\loss{\x}{\ptheta}}}$.
\end{theorem}

\begin{proof}
	Let $a_1=2(1-\gamma)\sig^2\alp$, ${a_2=\frac{1}{\gamma}\frac{S_g^2}{4n^2\sig^2}}$, $y=log(\q-1)$, and ${u(t,y)=\frac{R(\q,t)}{\q}-\frac{a_2}{a_1}}$.  We re-write \eqr{eqn:EvolvePDE} as the following form of transport with decay PDE
	\begin{equation*}
	\frac{\partial u}{\partial t}+a_1 u+a_1\frac{\partial u}{\partial y}\leq 0,
	\end{equation*}
	with initial condition $u(0,y)=-\frac{a_2}{a_1}$. By introducing variables $\tau=t$, and $z=t-\frac{1}{a_1} y$ and writing $v(\tau,z)=u(t,y)$, we get $\frac{\partial v}{\partial \tau}+a_1 v\leq0$, with initial condition ${v(0,z) = u(0,-a_1 z)}$.  For every $z$, this means that the decay of $v$ is proportional to its present value. The solution for this problem is ${v(\tau,z) \leq v(0,z)e^{-a_1 \tau}}$.  By bringing back the original variables, we have
	\begin{equation*}
	u(t,y)\leq u(0,y-a_1 t)e^{-a_1 t}.
	\end{equation*}
	
	Therefore,
	\begin{align*}
	R(\q,t)&\leq \frac{a_2}{a_1}(1-e^{-a_1 t})\\
    &=\frac{\q S_g^2}{8\gamma(1-\gamma) \alp n^2 \sig^4}(1-e^{-\sig^2\alp T})\\
    &=\frac{\q S_g^2}{2 \alp n^2 \sig^4}(1-e^{-\sig^2\alp T})\quad\text{set }\gamma=\frac{1}{2}.
	\end{align*}
\end{proof}

 \section{Proofs for privacy analysis of Noisy GD}
\label{sec:noisygdproof}

\begin{replemma}{lem:GDupdate_fokker}
    For SDE \eqr{eqn:discreteSDE}, the equivalent Fokker-Planck equation at time $\step\kk \leq t < \step(\kk+1)$ is
    \begin{equation}
        \doh{\rhO_t(\ptheta)}{t} = \divR{\left(\rhO_t(\ptheta)\Expec{\ptheta_\kk \sim \rhO_{\step\kk|t}}
        {\graD{\Loss_\D(\ptheta_\kk)|\ptheta}}\right)} + \tnoise^2\lapL{\rhO_t(\ptheta)},
    \end{equation}
    where the conditional distribution is defined as
    \begin{equation}
        \rhO_{\step\kk|t}(\ptheta|\ptheta') = \frac{\rhO_{\step\kk,t}(\ptheta, \ptheta')}{\rhO_t(\ptheta')}.
    \end{equation}
\end{replemma}

\begin{proof}
    Recall that conditionals of joint distribution $\rhO_{\step\kk,t}$ is 
    \begin{equation}
        \label{eqn:marg_cond}
        \rhO_{\step\kk,t}(\ptheta', \ptheta) = \rhO_{\step\kk}(\ptheta') \rhO_{t|\step\kk}(\ptheta|\ptheta') = \rhO_{t}(\ptheta) \rhO_{\step\kk|t}(\ptheta'|\ptheta).
    \end{equation}
    Marginalising away $\ptheta'$ in \eqr{eqn:marg_cond} and taking partial derivative w.r.t. $t$, we obtain the following.
    \begin{align*}
        &\doh{\rhO_t(\ptheta)}{t} = \int_{\thetaspace} \doh{\rhO_{t|\step\kk}(\ptheta|\ptheta')}{t}\rhO_{\step\kk}(\ptheta') \dif{\ptheta'} \\
        &\quad= \int_{\thetaspace} \left(\divR{\left(\rhO_{\step\kk,t}(\ptheta',\ptheta)\graD{\Loss_\D(\ptheta')}\right)} + \tnoise^2\lapL{\rhO_{\step\kk, t}(\ptheta', \ptheta)}\right) \dif{\ptheta'} \\
        &\quad=\divR{\left(\rhO_t(\ptheta)\int_{\thetaspace} \rhO_{\step\kk|t}(\ptheta'|\ptheta) \graD{\Loss_\D(\ptheta')\dif{\ptheta'}}\right)} + \tnoise^2\lapL{\rhO_t(\ptheta)} \\
        &\quad=\divR{\left(\rhO_t(\ptheta)\Expec{\ptheta' \sim \rhO_{\step\kk|t}}{\graD{\Loss_\D(\ptheta')}|\ptheta}\right)} + \tnoise^2\lapL{\rhO_t(\ptheta)}
    \end{align*}
\end{proof}

\begin{replemma}{lem:new_delayed_loss_diff}
    Let $\loss{\x}{\ptheta}$ be a $\be$-smooth loss function on closed convex set $\C$, with a finite total gradient sensitivity $\sen{\g}$, then for coupled tracing diffusions $\{\thet_t\}_{t\geq0}$ and $\{\thet_t'\}_{t\geq0}$ on neighboring datasets $\D, \D' \in \Domain$, under loss ${\smaloss{\x}{\ptheta}}$ and noise variance $\tnoise^2$, 
    the gradient sensitivity of conditionally expected loss is bounded by
    \begin{align}
        \Big\Vert\Expec{\ptheta_\kk\sim p_{\eta\kk|t}}{\graD{\Loss_{\D}(\ptheta_\kk)}\vert\ptheta} - &\Expec{\ptheta_\kk'\sim p'_{\eta\kk|t}}{\graD{\Loss_{\D'}(\ptheta_{\kk}')}\vert\ptheta}\Big\Vert_2^2 \leq \frac{S_g^2}{n^2(1-\step\be)^2}.
    \end{align}
\end{replemma}

\begin{proof}
    By definition of coupled tracing diffusion and \eqr{eqn:soldiscreteSDE}, we have for any $\tnoise^2$ and $\step$, the random variables $\thet_{\step\kk}, \thet_{\step\kk}', \thet_t, \thet_t'$ satisfy
    \begin{align}
        \label{eqn:new_delayed_update}
        \thet_{\step\kk} - (t-\step\kk) \graD{\Loss_\D(\thet_{\step\kk})} + \sqrt{2t\tnoise^2}\Z = \thet_t, \\
        \thet_{\step\kk}' - (t-\step\kk) \graD{\Loss_{\D'}(\thet_{\step\kk}')} + \sqrt{2t\tnoise^2}\Z' = \thet_t',
    \end{align}
    where $\Z, \Z' \sim \Gaus{0}{\Id}$, and $\kk$ is an integer s.t. ${\step\kk \leq t \leq \step(\kk+1)}$.

    We define the gradient descent update without noise on datasets $\D, \D'$ to be
    \begin{align}
        \phi(\ptheta)=I(\ptheta)-(t-\eta\kk)\nabla\Loss_{\D}(\ptheta), \\
        \phi'(\ptheta)=I(\ptheta)-(t-\eta\kk)\nabla\Loss_{\D'}(\ptheta),
    \end{align}
    where $I(\ptheta) = \ptheta$. By $\be$-smoothness of $\Loss_{\D}(\ptheta)$ and $\Loss_{\D'}(\ptheta)$, when $\be(t-\step\kk)<1$, for any $\ptheta_1,\ptheta_2\in\thetaspace$, we have
    \begin{align}
        \label{eqn:bilip}
        1-\eta\beta& \leq \frac{\norm{\phi(\ptheta_1)-\phi(\ptheta_2)}}{\norm{\ptheta_1-\ptheta_2}} \leq 1+\eta\beta,
    \end{align}
    and
    \begin{align}
        \label{eqn:bilip_1}
        1-\eta\beta & \leq \frac{\norm{\phi'(\ptheta_1)-\phi'(\ptheta_2)}}{\norm{\ptheta_1-\ptheta_2}} \leq 1+\eta\beta.
    \end{align}

    \textbf{Claim: $\phi$ and $\phi'$ is bijective.}

    \textbf{Proof:} \begin{enumerate}
        \item By \eqr{eqn:bilip}, $\norm{\phi(\ptheta_1)-\phi(\ptheta_2)}\geq (1-\eta\beta)\norm{\ptheta_1-\ptheta_2}$, $\therefore\phi$ is injective.
        \item Now we prove $\phi$ is surjective by proving its range $\phi(\thetaspace)=\thetaspace$.
        \begin{enumerate}
            \item We first prove $\phi(\thetaspace)$ is closed in $\thetaspace$. We only need to prove that any Cauchy sequence in $\phi(\thetaspace)$ converges to a point in $\phi(\thetaspace)$.  For any  $\{\phi(x_n)\}$ that is a cauchy sequence in $\phi(\thetaspace)$, by \eqr{eqn:bilip}, $\{x_n\}$ is also a cauchy sequence in $\thetaspace$, therefore ${\exists x\in\thetaspace}$, s.t. ${lim_{n\rightarrow\infty}x_n=x}$. By continuity of mapping $\phi$, ${lim_{n\rightarrow \infty}\phi(x_n)=\phi(lim_{n\rightarrow\infty}x_n)\in \mathbb{R}^d}$, therefore $\phi(\thetaspace)$ is closed.
            \item We then prove $\phi(\thetaspace)$ is open in $\thetaspace$. Since $\phi:\thetaspace\rightarrow\phi(\thetaspace)$ is injective continuous map, by invariance of domain theorem in topology, $\phi(\thetaspace)$ is an open set in $\thetaspace$.
            \item Since $\phi(\thetaspace)$ is closed and open in $\thetaspace$ and it's nonempty, we conclude that $\phi(\thetaspace)=\thetaspace$. That is $\phi$ is surjective. 
        \end{enumerate}
        \item Therefore $\phi$ is bijective.  Similarly we can prove $\phi'$ is bijective.
    \end{enumerate}
    
    Now we can define inverse $\psi=\phi^{-1}$, $\psi'=\phi'^{-1}$. 
    
    For any $\ptheta_3,\ptheta_4\in\thetaspace$, by \eqr{eqn:bilip}, we have
    \begin{align}
        \label{eqn:inverbilip}
        \frac{1}{1+\step\be}&\leq\frac{\norm{\psi(\ptheta_3)-\psi(\ptheta_4)}}{\norm{\ptheta_3-\ptheta_4}} \leq \frac{1}{1-\step\be},\\
        \frac{1}{1+\step\be}&\leq\frac{\norm{\psi'(\ptheta_3)-\psi'(\ptheta_4)}}{\norm{\ptheta_3-\ptheta_4}}\leq \frac{1}{1-\step\be}.
    \end{align}
    Suppose $\xi(\ptheta)=\phi'(\psi(\ptheta))$, then $\psi(\ptheta)=\psi'(\xi(\ptheta))$ and
    \begin{align}
        \xi(\ptheta)-\ptheta&=\phi'(\psi(\ptheta))-\phi(\psi(\ptheta))\\
        &=(t-\eta\kk)(\graD{\Loss_{\D'}(\psi(\ptheta))}-\graD{\Loss_{\D}(\psi(\ptheta))}).
    \end{align}
    Therefore,
    \begin{equation}
        \label{eqn:xirelation}\norm{\xi(\ptheta)-\ptheta}\leq (t-\eta\kk)\ \underset{\ptheta\in\thetaspace}{max}\ \norm{\graD{\Loss_{\D}(\ptheta)}-\graD{\Loss_{\D'}(\ptheta)}}
    \end{equation}
    Let the conditional gradient expectation $G(\ptheta) = \Expec{\ptheta_\kk\sim p_{\eta\kk|t}}{\graD{\Loss_{\D}(\ptheta_\kk)}\vert\ptheta} = \Expec{}{\graD{\Loss_{\D}(\thet_{\step\kk})}\vert \thet_t= \ptheta}$ be a function of $\ptheta$, and let ${G'(\ptheta) = \Expec{\ptheta_\kk'\sim p'_{\eta\kk|t}}{\graD{\Loss_{\D'}(\ptheta_{\kk}')}\vert\ptheta} = \Expec{}{\graD{\Loss_{\D'}(\thet_{\step\kk}')}\vert\thet_t'=\ptheta}}$. By \eqr{eqn:new_delayed_update} and~$\Expec{}{Z\vert\ptheta_t}=\Expec{}{Z'\vert\ptheta_t}$,  we have
    \begin{align*}  
        G(\ptheta) - G'(\ptheta)&=\frac{1}{t-\step\kk}\Expec{}{\thet_{\step\kk}-\thet_{\step\kk}'\vert\thet_t=\thet_t'=\ptheta}\\
        &=\frac{1}{t-\step\kk}\mathbb{E}[\psi(\ptheta+\sqrt{2\eta\sig^2}\Z)\\
        &\quad -\psi'(\ptheta+\sqrt{2\eta\sig^2}\Z')]\\
        &=\frac{1}{t-\eta\kk}\mathbb{E}[\psi'(\xi(\ptheta+\sqrt{2\step\sig^2}\Z))\\
        &\quad -\psi'(\ptheta+\sqrt{2\step\sig^2}\Z')]
    \end{align*}
    Note that since $\Z$ and $\Z'$ are i.i.d. gaussian standard noise, we can write the above as 
    \begin{align*}
        G(\ptheta) - G'(\ptheta)&=\frac{1}{t-\eta\kk}\mathbb{E}[\psi'(\xi(\ptheta+\sqrt{2\step\sig^2}\Z))\\
        &\quad -\psi'(\ptheta+\sqrt{2\step\sig^2}\Z)]
    \end{align*}
    where $\Z$ is standard gaussian noise. Note that
    \begin{align*}    
        \norm{\psi'(\xi(\ptheta))-\psi'(\ptheta)}
        &\leq \frac{\norm{\xi(\ptheta)-\ptheta}}{1-\step\be}\quad \tag{by \eqr{eqn:inverbilip}}\\
        &\leq\frac{(t-\eta\kk)\ \underset{\ptheta\in\thetaspace}{max}\ \norm{\graD{\Loss_{\D}(\ptheta)}-\graD{\Loss_{\D'}(\ptheta)}}}{1-\step\beta}. \tag{by \eqr{eqn:xirelation}}
    \end{align*}
    Therefore, we have for any $\theta\in\mathbb{R}^d$
    \begin{align*}
        \norm{G(\ptheta) - G'(\ptheta)}&\leq \frac{\norm{\graD{\Loss_{\D}(\ptheta+\sqrt{2\step\sig^2 } Z )}-\graD{ \Loss_{\D'}( \ptheta+\sqrt{2\step\sig^2}Z ) }}}{1-\eta\beta}\\
        \text{By definition of $S_g$}\quad&\leq \frac{S_g}{n(1-\eta\be)}.
    \end{align*}
\end{proof}

\begin{lemma}[ Rate of R\'enyi privacy loss ]
    \label{lem:marginalrenyidiscrete}
    Let $\{\thet_t\}_{t\geq 0}$ and $\{\thet_t'\}_{t\geq 0}$ be the coupled tracing 
    diffusions on neighboring datasets $\D,\D'\in\Domain$ for noisy GD under loss $\loss{\x}{\ptheta}$, noise variance $\sig^2$ and step-size $\step$.
    If loss function $\loss{\x}{\ptheta}$ is $\smh$-smooth, total gradient $g(\ptheta;\D)$ has finite sensitivity $\sen{\g}$, and the update step-size $\step<\frac{1}{\be}$, then for any $t \geq 0$, the rate of R\'enyi privacy loss of the tracing diffusion is upper bounded by
    \begin{align} 
        \negthickspace\negmedspace\doh{\Ren{\q}{\thet_t}{\thet_t'}}{t} \leq 
        \frac{1}{\gamma}\frac{\q \sen{\g}^2}{4\tnoise^2\size^2(1-\step\be)^2}-(1-\gamma)\frac{\tnoise^2\q}{2}\frac{\Gren{\q}{\thet_t}{\thet_t'}}{\Fren{\q}{\thet_t}{\thet_t'}}.
    \end{align}
    where $\gamma>0$ is a tuning parameter that we can fix arbitrarily according to our need.
\end{lemma}
    
\begin{proof}
    For brevity, let the functions ${R(\q,t)=\Ren{\q}{\rhO_{t}}{\rhO_{t}'}}$, ${E(\q,t)=\Fren{\q}{\rhO_{t}}{\rhO_{t}'}}$, and ${I(\q,t)=\Gren{\q}{\rhO_{t}}{\rhO_{t}'}}$. Following the same strategy as in proof of Lemma \ref{lem:marginalrenyi}, we can decompose $\doh{E(\q,t)}{t}$ using the Fokker-Planck equation \eqr{eqn:GDupdate_fokker} into
    \begin{equation*}
        \doh{E(\q,t)}{t} = F_1 + F_2,
    \end{equation*}
    where $F_1 = -\tnoise^2 \q(\q-1) I(\q, t)$ remains the same as in proof of Lemma \ref{lem:marginalrenyi}, but the second term $F_2$ is
    \begin{align*}
        F_2 &=\q\int_{\thetaspace}\left(\frac{\rhO_{t}}{\rhO_{t}'}\right)^{\q-1} \divR{(\rhO_{t}\Expec{}{\graD{\Loss_\D(\thet_{\step\kk})}|\ptheta_t})}\dif{\ptheta_t} \\
            &\quad -(\q-1)\int_{\thetaspace}\left(\frac{\rhO_{t}}{\rhO_{t}'}\right)^{\q} \divR{(\rhO_{t}'\Expec{}{\graD{\Loss_{\D}'(\thet_{\step\kk}')}|\ptheta_t})}\dif{\ptheta_t} \\
            &= (\q-1)\int_{\thetaspace}\dotP{\graD{\left(\frac{\rhO_{t}}{\rhO_{t}'}\right)^{\q}}}{\rhO_{t}' \underbrace{\Expec{}{\graD{\Loss_{\D'}(\thet_{\step\kk}')}|\ptheta_t}}_{= G'(\ptheta_t)}}\dif{\ptheta_t} \\
            &\quad -\q\int_{\thetaspace}\dotP{\graD{\left(\frac{\rhO_{t}}{\rhO_{t}'}\right)^{\q-1}}}{\rhO_{t}\underbrace{\Expec{}{\graD{\Loss_\D(\thet_{\step\kk})}|\ptheta_t}}_{= G(\ptheta_t)}}\dif{\ptheta_t}
            \tag{From \eqr{eqn:divr_dotp_eq}} \\
            &= \q(\q-1)\int_{\thetaspace}\left(\frac{\rhO_{t}}{\rhO_{t}'}\right)^{\q-2}\dotP{\graD{\frac{\rhO_{t}}{\rhO_{t}'}}}{\frac{\rhO_{t}}{\rhO_{t}'}G'(\ptheta_t)}\rhO_t'\dif{\ptheta_t}\\
            &\quad -\q(\q-1)\int_{\thetaspace}\left(\frac{\rhO_{t}}{\rhO_{t}'}\right)^{\q-2}\dotP{\graD{\frac{\rhO_{t}}{\rhO_{t}'}}}{\frac{\rhO_{t}}{\rhO_{t}'}G(\ptheta_t)}\rhO_t'\dif{\ptheta_t} \\
            &= \q(\q-1)\int_{\thetaspace}\negthickspace\left(\frac{\rhO_{t}}{\rhO_{t}'}\right)^{\q-2}\negthickspace\negthickspace\dotP{\negthickspace\graD{\frac{\rhO_{t}}{\rhO_{t}'}}}{\frac{\rhO_{t}}{\rhO_{t}'}\left(G'(\ptheta_t) - G(\ptheta_t)\right)\negthickspace}\rhO_t'\dif{\ptheta_t}
    \end{align*}
    Applying the trick (\eqr{eqn:young_ineq} with $b=2\gamma\tnoise^2$), we get
    \begin{align*}
        F_2 &\leq \gamma\tnoise^2 \q(\q-1)\int_{\thetaspace}\left(\frac{\rhO_{t}}{\rhO_{t}'}\right)^{\q-2}\norm{\graD{\frac{\rhO_{t}}{\rhO_{t}'}}}^2\rhO_{t}'\dif{\ptheta_t} \\
            &\quad + \frac{1}{\gamma}\frac{\q(\q-1)}{4\tnoise^2}\int_{\thetaspace}\left(\frac{\rhO_{t}}{\rhO_{t}'}\right)^{\q-2}\norm{\frac{\rhO_{t}}{\rhO_{t}'}\left(G'(\ptheta_t) - G(\ptheta_t)\right)}^2\rhO_{t}'\dif{\btheta} \\
            &\leq \gamma\tnoise^2 \q(\q-1) I(\q,t) + \frac{1}{\gamma}\frac{\q (\q-1)S_g^2}{4\tnoise^2\size^2(1-\step\be)^2} E(\q,t)
    \end{align*}
    Note that last inequality is from Lemma \ref{lem:new_delayed_loss_diff}, and the condition ${\step \leq \frac{1}{\smh}}$, which gives ${\vert\vert G(\ptheta_t) - G'(\ptheta_t)\vert\vert_2^2 \leq \frac{S_g^2}{\size^2(1-\step\be)^2}}$. We also substiute the integrals based on definitions in \eqr{eqn:frenyi_divergence} and \eqr{eqn:grenyi_divergence}.
    Finally, just like in Lemma \ref{lem:marginalrenyi} we get
    \begin{align*}
        \doh{R(\q,t)}{t}&=\frac{1}{\q-1}\times \frac{1}{E(\q,t)}\times\doh{E(\q,t)}{t}\\
                        &\leq -\gamma\tnoise^2 \q\frac{I(\q,t)}{E(\q,t)} + \frac{1}{\gamma}\frac{\q S_g^2}{4\tnoise^2\size^2(1-\step\be)^2} 
    \end{align*}
\end{proof}

    % \begin{reptheorem}{thm:RDbounddiscrete}[RDP for noisy GD under $\alp$-LSI]
    %      %
    % Let $\{\thet_t\}_{t\geq0}$ be the tracing diffusion for $\algo_{\text{Noisy-GD}}$ on dataset $\database$. Assume the loss function $\loss{\x}{\ptheta}$ is $\be$-smooth and total gradient $g(\ptheta;\D)$ has a finite sensitivity $\sen{\g}$. 
    
    % If for any $\D$, the distribution of $\thet_{t}$ satisfies $\alp$-LSI throughout ${0\leq t\leq \step\K}$, and the update step-size $\step< \frac{1}{\be}$, then $\algo_{\text{Noisy-GD}}$ satisfies $(\q, \eps)$ R\'enyi DP for
    % %
    % \begin{equation} 
    %     \eps \geq \frac{\q \sen{\g}^2}{2\alp\sig^4\size^2(1-\step\be)^2}(1-e^{-\sig^2\alp\step\K})
    % \end{equation}
    % \end{reptheorem}
    
    % \begin{proof}
    %     For every time interval ${\kk\step\leq t<(\kk+1)\step}$, the same PDE \eqr{eqn:evolvePDEdiscrete} applies under the stated assumptions. Therefore, we can solve the PDE directly for the entire duration $0 \leq t \leq \K\step$ almost identically as the proof of theorem \ref{thm:RDboundCD}, with a slight modification that constant ${a_2=\frac{\sen{\g}^2}{2\alp\sig^4\size^2(1-\step\be)^2}}$. This results in an RDP guarantee for noisy GD.
    % \end{proof}

\begin{reptheorem}{thm:RDbounddiscrete}
    Let $\{\thet_t\}_{t\geq0}$ be the tracing diffusion for $\algo_{\text{Noisy-GD}}$ on dataset $\database$. Let $\loss{\x}{\ptheta}$ be a $\be$-smooth loss function on closed convex set $\C$, with a finite total gradient sensitivity $\sen{\g}$. 
    If $\thet_{t}$ satisfies $\alp$-LSI throughout ${0\leq t\leq \step\K}$, and the step-size $\step< \frac{1}{\be}$, then $\algo_{\text{Noisy-GD}}$ satisfies $(\q, \eps)$ R\'enyi Differential Privacy for
    \begin{equation} \label{eqn:RDbounddiscrete}
        \eps = \frac{\q \sen{\g}^2}{2\alp\sig^4\size^2(1-\step\be)^2}(1-e^{-\sig^2\alp\step\K})
    \end{equation}
\end{reptheorem}

\begin{proof}
    % The proof is similar to similar to that of Theorem~\ref{thm:RDboundCD} for coupled diffusion under the same finite total gradient sensitivity $S_g$ and $\alp$-LSI condition, except for dealing with the projection step. We only provide a sketch of proof. 
    
    The RDP evolution equation ~\ref{eqn:evolvePDEdiscrete} holds for projected noisy GD during the tracing diffusion in every time piece $\step\kk\leq t<\step(\kk+1)$. Therefore, we have

    \begin{equation*}
        \doh{R(\q,t)}{t} 
        \leq
        \frac{1}{\gamma}\frac{\q \sen{\g}^2}{4\tnoise^2\size^2(1-\step\be)^2}
        - 2(1-\gamma)\sig^2\alp \left[ \frac{R(\q,t)}{\q}     
        + (\q-1)\frac{\partial R(\q,t)}{\partial\q} \right]
    \end{equation*}
    
    Let $a_1=2(1-\gamma)\sig^2\alp$, ${a_2=\frac{1}{\gamma}\frac{S_g^2}{4\sig^2n^2(1-\step\be)^2}}$, $y=log(\q-1)$, and ${u(t,y)=\frac{R(\q,t)}{\q}-\frac{a_2}{a_1}}$.  We re-write \eqr{eqn:EvolvePDE} as the following form of transport with decay PDE
	\begin{equation*}
	\frac{\partial u}{\partial t}+a_1 u+a_1\frac{\partial u}{\partial y}\leq 0,
	\end{equation*}
	with initial condition $u(\step\kk,y)=\frac{R(\q,\step\kk)}{\q}-\frac{a_2}{a_1}$. By introducing variables $\tau=t$, and $z=t-\frac{1}{a_1} y$ and writing $v(\tau,z)=u(t,y)$, we get $\frac{\partial v}{\partial \tau}+a_1 v\leq0$, with initial condition ${v(\step\kk,z) = u(\step\kk,-a_1 (z-\step\kk))}$.  For every $z$, this means that the decay of $v$ is proportional to its present value. The solution for this problem is ${v(\tau,z) \leq v(\step\kk,z)e^{-a_1 (\tau-\step\kk)}}$.  By bringing back the original variables, we have
	\begin{equation*}
	u(t,y)\leq u(\step\kk,y-a_1 (t-\step\kk))e^{-a_1 (t-\step\kk)}.
	\end{equation*}
	
	Further bringing back the original $R(\q,t)$ variables, we have
	\begin{align*}
	R(\q,t)-\frac{a_2}{a_1}\q&\leq (R(\q,\step\kk)-\frac{a_2}{a_1}\q)e^{-a_1 (t-\step\kk)}\\
	\end{align*}

    Taking limit $t\rightarrow\step(\kk+1)$, where $\step\kk\leq t<\step(\kk+1)$, we have
    \begin{align*}
        \lim_{t\rightarrow\step(\kk+1)}R(\q,t)-\frac{a_2}{a_1}\q&\leq (R(\q,\step\kk)-\frac{a_2}{a_1}\q)e^{-a_1 \step}\\
    \end{align*}

    Because $\thet_{\step(\kk+1)}=\proj{\C}{\lim_{t\rightarrow\step(\kk+1)}\thet_t}$, and projection is post-processing which preserves privacy, 
    \begin{equation*}
        R(\q,\step(\kk+1))-\frac{a_2}{a_1}\q\leq \lim_{t\rightarrow\step(\kk+1)}R(\q,t)-\frac{a_2}{a_1}\q
    \end{equation*}
    
    Combining the above two inequalities, we immediately have the following recursive equation,
    \begin{equation*}
        R(\q,\step(\kk+1))-\frac{a_2}{a_1}\q\leq(R(\q,\step\kk)-\frac{a_2}{a_1}\q)e^{-a_1 \step}\\
    \end{equation*}
    
    Repeating this step for $\kk=0,\cdots,\K-1$ we have
    \begin{equation*}
        R(\q,\step\K)-\frac{a_2}{a_1}\q\leq(R(\q,0)-\frac{a_2}{a_1}\q)e^{-a_1 \step\K}\\
    \end{equation*}
    
    Because coupled tracing diffusion have the same start parameter, we have $R(\q,0)=0$.

    Therefore, taking the value $a_1=2(1-\gamma)\sig^2\alp$, ${a_2=\frac{1}{\gamma}\frac{S_g^2}{4\sig^2n^2(1-\step\be)^2}}$ into the equation, we have
    \begin{equation*}
        R(\q,\step\K)\leq \frac{\q \sen{\g}^2}{8\gamma(1-\gamma)\alp\sig^4\size^2(1-\step\be)^2}(1-e^{-2(1-\gamma)\sig^2\alp\step\K})
    \end{equation*}

    Setting $\gamma=\frac{1}{2}$ suffices to prove the R\'enyi privacy loss bound in the theorem.
\end{proof}
    
This R\'enyi differential privacy bound has quadratic dependence on the total gradient sensitivity $S_g$, which can upper bounded $S_g\leq 2\Lip$ when the loss function is $\Lip$-Lipschitz, which matches the RDP guarantees in the prior work~\cite{abadi2016deep, feldman2018privacy}.  As discussed before, here the convex set $\C$ is implicitly contrained to be bounded due to Lipschitzness and strong convexity. Morover, the strong convexity parameter $\lambda$ must be smaller than the smoothness parameter $\beta$ due to definition.

 \input{appendices/tightness_proof.tex}
 \input{appendices/projectionproof.tex}
