# Supplementary material for: Differential Privacy Dynamics of Langevin Diffusion and Noisy Gradient Descent
Source: arXiv:2102.05855 source file (2022-09-09)
Supplement: Supplementary file 2 [file appendix_more_discussion.tex]

\section{More Discussions of results}

\subsection{Novelty of this paper}
Our privacy erosion dynamics analysis for noisy GD is motivated by the rapid convergence analysis for ULA in \citet{vempala2019rapid}. However, because our algorithm noisy GD is slightly different from ULA and we focus on the privacy context, there are many \textbf{technical differences} between our approach and that of \citet{vempala2019rapid}.
\begin{enumerate}
    \item \textbf{Different divergence objective analyzed:} In \citet{vempala2019rapid}, they analyze \textbf{convergence guarantee} of ULA process, and bound the Rényi divergence between the \emph{$k$-th step distribution in ULA} and its \textbf{biased stationary distribution}. However, our paper analyzes the \textbf{privacy bound}, and bounds a \emph{different} Rényi divergence between the \emph{$k$th step distributions} of \emph{two noisy GD processes} running on neighboring datasets $D,D'$.
    
    The Rényi divergence analyzed in \citet{vempala2019rapid} is between one ULA process and its biased stationary distribution, which is \textbf{different from} the Rényi privacy loss $R_{\alpha}(\thet_t\lVert\thet_t')$ analyzed in our paper. As a result, we prove converging privacy loss \textbf{without assuming or utilizing the convergence of individual noisy GD process} to its stationary distribution in Rényi divergence, while this assumption is made and proved in \citet{vempala2019rapid}. 
    
    The Rényi divergence analyzed in \citet{vempala2019rapid} only involves \textbf{one evolving ULA process} and a \textbf{static stationary distribution} of ULA. However, the privacy loss divergence analyzed in our paper analyzes \textbf{two evolving noisy GD processes} running on neighboring datasets $D,D'$. This is technically more difficult than \citet{vempala2019rapid} because we use the SDEs for tracing diffusions of two simultaneously evolving noisy GD processes. 
    
    The convergence of privacy loss divergence analyzed in our paper requires \textbf{a slightly different LSI constant condition} than that in \citet{vempala2019rapid}. The convergence guarantee of one ULA process in Lemma 8 of \citet{vempala2019rapid} only requires LSI constant bound for the \textbf{biased stationary distribution}. On the contrary, our privacy analysis requires LSI constant bound \textbf{throughout the tracing diffusion processes}, for two noisy GD processes running on neighboring datasets $D,D'$. Our LSI constant condition throughout tracing diffusion is different from, as well as more difficult to satisfy, than the LSI condition for stationary distribution in \citet{vempala2019rapid}.
    \item \textbf{Different algorithms analyzed:} We analyze \textbf{Projected Noisy GD algorithm}, while \citet{vempala2019rapid} analyzes \textbf{ULA} (equivalent to Noisy GD \textbf{without projection}). Due to the additional projection operation, our tracing diffusion is semi-continous, while the underlying diffusion in \citet{vempala2019rapid} for ULA updates is continuous. Therefore, our divergence analysis handles the additional complexity due to the \textbf{semi-continuity in the tracing diffusion}. 
\end{enumerate}

To conclude, we summarize our \textbf{novelties} in comparison with \citet{vempala2019rapid} as follows.
\begin{enumerate}
    \item \textbf{Novel privacy bound for projected noisy GD in Rényi divergence} 
    
    We prove a novel bound for the \textbf{rate of privacy loss} in Lemma~\ref{lem:marginalrenyi} for the tracing diffusion processes underlying projected noisy GD algorithms, which is not proved in \citet{vempala2019rapid}. Our derivation of the rate of Rényi privacy loss for diffusion processes is new and novel. Other than our work, we are only aware of a similar entropy production formula ( Lemma 3.1 of \citet{olla1993hydrodynamical}, originated from \citet{yau1991relative}) for KL divergence, which bounds the rate of KL divergence between any two stochastic processes, with terms determined by the partial derivative of base probability density with regard to time $t$. This shares a similar form with our \eqr{eqn:marginalrenyi}. Our novelty is to calculate this rate of Rényi divergence, with arbitrary order $\alpha$, for Langevin diffusion processes.
    
    We prove a novel \textbf{converging privacy bound for noisy GD} in Theorem~\ref{thm:RDbounddiscrete} under LSI condition, without assuming that the noisy GD process converges to a stationary distribution. However, the convergence guarantee of Lemma 8 in \citet{vempala2019rapid} requires smoothness of the loss function and the LSI assumption, and proves that single ULA process converge to a stationary distribution. 
    
    \item \textbf{Novel LSI constant bound throughout Noisy GD} 
    
    In Lemma \ref{lem:iso_convex}, we also prove a novel \textbf{LSI constant bound} for distributions \textbf{throughout} the tracing diffusion of projected noisy GD, under smooth strongly convex loss functions. Meanwhile, \citet{vempala2019rapid} assumes LSI constant bound only for the \textbf{stationary distribution} of ULA, and do not prove this LSI condition under any practical settings.
\end{enumerate}

\subsection{More discussions about relaxing conditions for privacy dynamics analysis}

Our privacy dynamics analysis relies on two important conditions: smooth strongly convex loss functions and full gradient update. We now discuss the open problem of relaxing these conditions for privacy dynamics analysis.

\paragraph{Relaxing the assumption of strongly convex smooth loss functions}

This is an important problem. Some assumptions in our analysis impose technical difficulties, for which the results in the literature for non-convex loss functions \textbf{cannot be used in a straight-forward manner} (to the best of our knowledge). We understand these assumptions may limit the application of our analysis, however, we view our current analysis for strongly convex and smooth loss as a first major step towards privacy analysis for black-box noisy GD under \textbf{more complex loss functions}. To extend our analysis to the general non-convex non-smooth loss function, we believe the key t\textbf{technical challenges} are the following.
\begin{enumerate}
    \item \textbf{Adding appropriate conditions for loss functions:} To our knowledge, obtaining general divergence bounds for distributions under non-convex loss functions is very difficult. Therefore, existing works often make various additional assumptions to facilitate analysis. This includes dissipative condition in \citet{raginsky2017non}, Hessian Lipschitz condition in \citet{vempala2019rapid}, and Boundedness loss condition in \citet{li2019generalization}.
    \item \textbf{Bounding the LSI constant throughout tracing diffusions:} Although our privacy bound Theorem ~\ref{thm:RDbounddiscrete} holds for noisy GD under non-convex loss function, bounding the LSI constant $c$ is another technical challenge. Previously, many results, such as \citet{raginsky2017non}, prove LSI constant bound for the \textbf{stationary Gibbs distribution} of SGLD under non-convex loss. However, our framework requires a \textbf{stricter} LSI constant bound \textbf{throughout} the tracing diffusion processes, which poses new technical challenges. We are only aware of one such result in \citet{li2019generalization} for SGLD on bounded loss with $\ell_2$-regularization. 
\end{enumerate}

\paragraph{Relaxing full gradient update to stochastic gradient update} 

Extending our privacy analysis for (noisy) SGD updates would be an important future work, and there are multiple technical challenges to overcome. 

The more achievable way to extend our privacy analysis to noisy SGD lies in the \textbf{privacy amplification by sampling} literature, e.g. \citet{mironov2019r}, which prove that the privacy loss for one SGD update is smaller than the privacy loss of a full-batched GD update by squared sampling ratio. However, our analysis requires quantifying the privacy amplification of multiple SGD updates with iterative re-sampling, which is technically more involved and requires new results.

A more difficult way is to \textbf{analyze the privacy erosion for the new (noisy) SGD process}, which poses the following technical challenges.
\begin{enumerate}
    \item \textbf{Variety of methods to sample mini-batches from the dataset:} Various sampling methods, such as sampling \emph{without replacement}, sampling \emph{with replacement}, \emph{Poisson} sampling, and the most commonly used \emph{shuffle than partition}, result in different processes during (noisy) SGD update. They often requiring separate privacy analyses.
    \item \textbf{Deriving the \emph{exact} SDE for (noisy) SGD updates:} To the best of our knowledge, the existing literature which uses underlying continuous diffusion processes to trace the (noisy) SGD updates, e.g. in \citet{raginsky2017non} and \citet{li2019generalization}, usually has approximation error that depends on the discretization step-size $\eta$. Meanwhile, our current privacy analysis would require an underlying diffusion process that \textbf{exactly} interpolates the discrete SGD updates, and therefore cannot use these approximate SDEs straightforwardly. To extend our analysis to (noisy) SGD, we either need the \textbf{exact} underlying SDE for noisy SGD, or a \textbf{new} privacy erosion analysis technique based on \textbf{approximate SDE}, which both require more technical investigations.
    \item \textbf{Bounding LSI constant throughout tracing diffusion}. Our privacy bound relies on the LSI constant throughout the tracing diffusion process. Meanwhile, previous papers, such as \citet{raginsky2017non}, only require and prove LSI constant bounds for the stationary Gibbs distribution of SGLD. To our knowledge, for general intermediate distribution in SGLD, it is difficult to prove a (tight) bound on the LSI constant $c$. We are only aware of one such result in \citet{li2019generalization} for SGLD on bounded loss with $\ell_2$-regularization. 
\end{enumerate}
