# Supplementary material for: Differential Privacy Dynamics of Langevin Diffusion and Noisy Gradient Descent
Source: arXiv:2102.05855 source file (2022-09-09)
Supplement: Supplementary file 3 [file LSI.tex]

\section{Proof techniques for log-Sobolev inequality}

\label{sec:appendixLSI}

As mentioned before, the literature on LSI is rich with a variety of techniques used to prove this inequality for several kinds of distributions. To prove that LSI holds for the tracing diffusion, we rely on the following two lemmas that show Lipschitz transformation and Gaussian perturbation of a probability distribution preserve its LSI property.

\begin{lemma}[LSI under Lipschitz transformation~\cite{ledoux2001concentration}]
    \label{lem:lip_lsi}
    Suppose a probability distribution $\rhO$ on $\thetaspace$ satisfies LSI with constant~$\alp > 0$.  Let $T:\thetaspace \rightarrow \thetaspace$ be a differentiable and $\lip$-Lipschitz transformation. The push-forward distribution~$T_{\#\rhO}$, representing $T(\thet)$ when $\thet \sim \rhO$, satisfies LSI with constant~$\frac{\alp}{\lip^2}$.
\end{lemma}

\begin{lemma}[LSI under Gaussian convolution~\cite{ledoux2001concentration}]
    \label{lem:gaus_conv_lsi}
    Suppose a probability distribution $\rhO$ on $\thetaspace$ satisfies LSI with constant~${\alp > 0}$.  For $t>0$, the probability distribution $\rhO * \Gaus{0}{2t\Id}$ satisfies LSI with constant~$\left(\frac{1}{\alp} + 2t\right)^{-1}$. A special case of this is that $\Gaus{0}{2t\Id}$ satisfies LSI with constant~$\frac{1}{2t}$.
\end{lemma}

\begin{replemma}{lem:iso_convex}
    If loss function $\loss{\x}{\ptheta}$ is $\cvx$-strongly convex and $\smh$-smooth over a closed convex set $\C$, the step-size is ${\step < \frac{1}{\smh}}$, and initial distribution is $\thet_{0} \sim \proj{\C}{\Gaus{0}{\frac{2\tnoise^2}{\cvx}\Id}}$, then the distribution of tracing diffusion~$\thet_t$ for noisy GD satisfies $\alp$-LSI for any $t\geq0$ with 
    \begin{equation*}
        \alp=\frac{\lam}{2\sig^2}.
    \end{equation*}
 \end{replemma}
 
 \begin{proof}
     For any $\D \in \Domain$, and $0\leq s\leq\step$, define the update step in \alg{alg:noisygd} to be the mapping ${T(\ptheta)=\proj{\C}{ T_1(\ptheta)}}$, where ${T_1(\ptheta)=\ptheta- s\graD{\Loss_\D(\ptheta)}}$. We first show that $T_1$ is $(1-s\cvx)$-Lipschitz. For any $w, v \in \thetaspace$, we have
     \begin{align*}
         T_1(w)-T_1(v) &= w-v-s(\graD{\Loss_\D(w)}-\graD{\Loss_\D(v)})\\
         &=w-v- s\hesS{\Loss_\D(z)}(w-v) \tag{for some $z \in \thetaspace$ due to M.V.T}\\
         &=(I-s\hesS{\Loss_\D(z)})(w-v)
     \end{align*}  
     By convexity and $\smh$-smoothness, $\hesS{\Loss_\D}$ has eigenvalue in $[\cvx,\smh]$. Since $s \leq \step\leq \frac{1}{\smh}$, all eigenvalues of $(I- s\graD{\Loss_\D})$ is in $[0,1-s\cvx]$, so $T_1$ is $(1-s\cvx)$-Lipshitz. 
     
     Now, using induction we prove $\rhO_t$ statisfies $\alp$-LSI for $\alp=\frac{\cvx}{2\tnoise^2}$ for any $t \geq 0$. 
     
     {\bf Base step:} Being a Gaussian with variance $\frac{\cvx}{2\tnoise^2}$, $\rhO_0$ satisfies $\alp$-LSI with the given constant as per lemma \ref{lem:gaus_conv_lsi}.    
 
     {\bf Induction step:} Suppose $\rhO_{\step\kk}$ satisfies $\alp$-LSI with the above constant for some $k \in \N$. Distribution $\rhO_{t}$ for ${\step \kk \leq t < \step (\kk+1)}$ is same as $T$ pushover distribution plus gaussian noise distribution, i.e.  ${\rhO_t = \rhO_{\step \kk}}_{\# T} * \Gaus{0}{2s\tnoise^2\Id}$ for $s = t - \step \kk$. Using lemma \ref{lem:lip_lsi} and \ref{lem:gaus_conv_lsi}, we get
     $\left( \frac{\alp}{(1 - s\cvx)^2 + 2s\tnoise^2\alp} \right)$-LSI for $\rhO_t$.
     Since $s \leq \step \leq \frac{1}{\cvx}$, we have
     \begin{equation*}
         (1-s\cvx)^2 + 2s\tnoise^2\alp \leq 1 - s\cvx + 2s\tnoise^2\alp = 1.
     \end{equation*}
     So for $\eta\kk\leq t<\eta(\kk+1)$, $\rhO_{t}$ satisfies $\alp'$-LSI with constant $\alp' \geq \alp$, which by definition also satisfies $\alp$-LSI.
     For $t=\eta(\kk+1)$, $p_{(k+1)\eta}=$ is same as projected $T$ pushover distribution plus gaussian noise distribution. We've already proved that $T$ pushover distribution plus gaussian noise distribution still satisfies $\alp$-LSI. And since projection is a 
     $1$-Lipschitz map, by Lemma \ref{lem:lip_lsi}, it preserves $\alp$-LSI. So distribution $p_{(k+1)\eta}$ satisfies $\alp$-LSI.
 \end{proof}
