# Supplementary material for: Differential Privacy Dynamics of Langevin Diffusion and Noisy Gradient Descent
Source: arXiv:2102.05855 source file (2022-09-09)
Supplement: Supplementary file 5 [file diffusion_proofs.tex]

\section{Proofs for privacy analysis of Langevin Diffusion}
\label{sec:diffusion_proof}

\begin{replemma}{lem:marginalrenyi}[ Rate of R\'enyi Privacy Loss ]
Let $\loss{\x}{\ptheta}$ be a loss function on $\thetaspace$, with a finite total gradient sensitivity $\sen{\g}$. Then for coupled Langevin diffusions $\{\thet_t\}_{t\geq0}$ and $\{\thet_t'\}_{t\geq0}$ on neighboring datasets $\D, \D' \in \Domain$, under loss ${\smaloss{\x}{\ptheta}}$ and noise variance $\tnoise^2$, the R\'enyi privacy loss rate at any $t\geq0$ is upper bounded by
\begin{equation}
    \doh{\Ren{\q}{\thet_{t}}{\thet_{t}'}}{t}
    \leq 
    \frac{1}{\gamma}\frac{\q S_g^2}{4\tnoise^2\size^2}
    -
    (1-\gamma)\tnoise^2\q \frac{\Gren{\q}{\thet_{t}}{\thet_{t}'}}{\Fren{\q}{\thet_{t}}{\thet_{t}'}}.
\end{equation}
where $\gamma>0$ is a tuning parameter that we can fix arbitrarily according to our need.
\end{replemma}

\begin{proof}
    For brevity, let the functions ${R(\q,t)=\Ren{\q}{\rhO_{t}}{\rhO_{t}'}}$, ${E(\q,t)=\Fren{\q}{\rhO_{t}}{\rhO_{t}'}}$, and ${I(\q,t)=\Gren{\q}{\rhO_{t}}{\rhO_{t}'}}$. Under the stated assumptions $\doh{E(\q,t)}{t}$ is bounded as follows.
    \begin{align*}
        \doh{E(\q,t)}{t} &=\doh{}{t}\int_{\thetaspace}\frac{\rhO_{t}^{\q}}{\rhO_{t}'^{\q-1}}\dif{\ptheta} \\
        &= \q \int_{\thetaspace} \doh{\rhO_{t}}{t} \left(\frac{\rhO_{t}}{\rhO_{t}'}\right)^{\q-1}\dif{\ptheta} \\
        &\quad    -(\q-1) \int_{\thetaspace} \doh{\rhO_{t}'}{t} \left(\frac{\rhO_{t}}{\rhO_{t}'}\right)^{\q} \dif{\ptheta} \\
        &=\ \q\int_{\thetaspace} \left(\tnoise^2\lapL{\rhO_{t}} + \divR{(\rhO_{t}\graD{\Loss(\D)})}\right)
            \left(\frac{\rhO_{t}}{\rhO_{t}'}\right)^{\q-1}\dif{\ptheta} \\
        &\quad -(\q-1)\int_{\thetaspace} \big(\tnoise^2\lapL{\rhO_{t}'}+ \divR{(\rhO_{t}'\graD{\Loss(\D')})}\big) \\
        & \quad\quad\quad\quad\quad\quad\quad\quad\quad
            \left(\frac{\rhO_{t}}{\rhO_{t}'}\right)^\q\dif{\ptheta}
            \tag{From \eqr{eqn:fokkerplanck}} \\
        &   \begin{rcases}
                =\tnoise^2 \q\int_{\thetaspace}\left(\frac{\rhO_{t}}{\rhO_{t}'}\right)^{\q-1}\lapL{\rhO_{t}}\dif{\ptheta} \\
                \quad -\tnoise^2(\q-1)\int_{\thetaspace}\left(\frac{\rhO_{t}}{\rhO_{t}'}\right)^{\q}\lapL{\rhO_{t}'}\dif{\ptheta}
            \end{rcases} \eqdef F_1 \\
        &   \begin{rcases}  
                \quad +\q\int_{\thetaspace}\left(\frac{\rhO_{t}}{\rhO_{t}'}\right)^{\q-1} \divR{(\rhO_{t}\graD{\Loss(\D)})}\dif{\ptheta} \\
                \quad -(\q-1)\int_{\thetaspace}\left(\frac{\rhO_{t}}{\rhO_{t}'}\right)^{\q} \divR{(\rhO_{t}'\graD{\Loss(\D')})}\dif{\ptheta}
            \end{rcases} \eqdef F_2
    \end{align*}
    Now $F_1$ is equivalent to the following.
    \begin{align*}
        F_1 &= \tnoise^2(\q-1)\int_{\thetaspace}\dotP{\graD{\left(\frac{\rhO_{t}}{\rhO_{t}'}\right)^\q}}{\graD{\rhO_{t}'}}\dif{\ptheta} \\
            &\quad -\tnoise^2 \q\int_{\thetaspace}\dotP{\graD{\left(\frac{\rhO_{t}}{\rhO_{t}'}\right)^{\q-1}}}{\graD{\rhO_{t}}}\dif{\ptheta}
                \tag{From \eqr{eqn:lapl_dotp_eq}} \\
            &= \tnoise^2 \q(\q-1)\int_{\thetaspace} \negthickspace\left(\frac{\rhO_{t}}{\rhO_{t}'}\right)^{\q-2}\negthickspace\negthickspace\dotP{\negthickspace\graD{\frac{\rhO_{t}}{\rhO_{t}'}}}
                {\frac{\rhO_{t}}{\rhO_{t}'^2}\graD{\rhO_{t}'} - \frac{\graD{\rhO_{t}}}{\rhO_{t}'}\negthickspace}\rhO_{t}'\dif{\ptheta} \\
            &= -\tnoise^2 \q(\q-1)\Expec{\rhO_{t}'}{\left(\frac{\rhO_{t}}{\rhO_{t}'}\right)^{\q-2} \norm{\graD{\frac{\rhO_{t}}{\rhO_{t}'}}}^2}
                \tag{$\because \graD{\frac{\rhO_{t}}{\rhO_{t}'}} = \frac{\graD{\rhO_{t}}}{\rhO_{t}'} - \frac{\rhO_{t}}{\rhO_{t}'^2}\graD{\rhO_{t}'}$} \\
            &= -\tnoise^2 \q(\q-1) I(\q, t) \tag{From \eqr{eqn:grenyi_divergence}}
    \end{align*}
    And $F_2$ is upper bounded by the following.
    \begin{align*}
        F_2 &= (\q-1)\int_{\thetaspace}\dotP{\graD{\left(\frac{\rhO_{t}}{\rhO_{t}'}\right)^{\q}}}{\rhO_{t}' \graD{\Loss(\D')}}\dif{\ptheta} \\
            &\quad -\q\int_{\thetaspace}\dotP{\graD{\left(\frac{\rhO_{t}}{\rhO_{t}'}\right)^{\q-1}}}{\rhO_{t}\graD{\Loss(\D)}}\dif{\ptheta}
                \tag{From \eqr{eqn:divr_dotp_eq}} \\
            &= \q(\q-1)\negthickspace\int_{\thetaspace}\negthickspace\left(\frac{\rhO_{t}}{\rhO_{t}'}\right)^{\q-2}\negthickspace\negthickspace\dotP{\negthickspace\graD{\frac{\rhO_{t}}{\rhO_{t}'}}}
                {\frac{\rhO_{t}}{\rhO_{t}'}\graD{\left(\Loss(D') - \Loss(D)}\right)\negthickspace}\rhO_{t}'\dif{\ptheta} \\
            &\leq \gamma \q(\q-1)\tnoise^2\int_{\thetaspace}\left(\frac{\rhO_{t}}{\rhO_{t}'}\right)^{\q-2}\norm{\graD{\frac{\rhO_{t}}{\rhO_{t}'}}}^2\rhO_{t}'\dif{\ptheta}
                \tag{From \eqr{eqn:young_ineq} with $b=2\gamma\tnoise^2$} \\
            &\quad + \frac{\q(\q-1)}{4\gamma\tnoise^2}\left(\frac{S_g}{\size}\right)^2\int_{\thetaspace}\left(\frac{\rhO_{t}}{\rhO_{t}'}\right)^{\q-2}\norm{\frac{\rhO_{t}}{\rhO_{t}'}}^2\rhO_{t}'\dif{\ptheta}
                \tag{$\because {\vert\vert\graD{\smaloss{\x}{\ptheta}}-\graD{\smaloss{\x'}{\ptheta}}\vert\vert_2\leq S_g}$ by definition} \\
            &\leq \gamma\tnoise^2 \q(\q-1) I(\q,t) + \frac{1}{\gamma}\frac{\q(\q-1)S_g^2}{4\tnoise^2\size^2} E(\q,t) \tag{From \eqr{eqn:frenyi_divergence} \& \eqr{eqn:grenyi_divergence}}
    \end{align*}
    Therefore, we get the following bound on the rate of Renyi divergence.
    \begin{align*}
        \doh{R(\q,t)}{t}&=\frac{1}{\q-1}\times \frac{1}{E(\q,t)}\times\doh{E(\q,t)}{t}\\
                                                &\leq -(1-\gamma)\tnoise^2 \q\frac{I(\q,t)}{E(\q,t)} + \frac{1}{\gamma}\frac{\q S_g^2}{4\tnoise^2\size^2} 
    \end{align*}
\end{proof}

\begin{replemma}{lem:RDinLSI}[ $\alp$-LSI in terms of Rényi Divergence~\cite{vempala2019rapid} ]
    Suppose $\rhO,\rhO'$ are probability distributions of random variables $\thet_t, \thet_t'$ on $\thetaspace$. If $\frac{\rhO}{\rhO'}\in\Ftheta{\thet_t'}$, 
    then for any $\q \geq 1$, 
    \begin{align*} 
        \Ren{\q}{\thet_t}{\thet_t'} 
        + 
        \q(\q - 1) \doh{\Ren{\q}{\thet_t}{\thet_t'}}{\q}  
        \leq 
        \frac{\q^2}{2\alp} \frac{\Gren{\q}{\thet_t}{\thet_t'}}{\Fren{\q}{\thet_t}{\thet_t'}},
    \end{align*}
    if and only if $\rhO'$ satisfies $\alp$-LSI.
\end{replemma}

\begin{proof}
    For brevity, let the functions ${R(\q)=\Ren{\q}{\thet_t}{\thet_t'}}$, ${E(\q)=\Fren{\q}{\thet_t}{\thet_t'}}$, and ${I(\q)=\Gren{\q}{\thet_t}{\thet_t'}}$. 
    Let function ${g^2(\ptheta)=\left(\frac{\rhO(\ptheta)}{\rhO'(\ptheta)}\right)^\q}$. Then,
    \begin{align*}
        \Expec{\rhO'}{g^2} = \Expec{\rhO'}{\left(\frac{\rhO}{\rhO'}\right)^{\q}} = \Frenyi{\q}{\rhO}{\rhO'},
        \tag{From \eqr{eqn:frenyi_divergence}}
    \end{align*}
    and,
    \begin{align*}
        \Expec{\rhO'}{g^2 \log g^2} &= \Expec{\rhO'}{\left(\frac{\rhO}{\rhO'}\right)^{\q} 
                                   \log \left(\frac{\rhO}{\rhO'}\right)^{\q}} \\
                                   &= \q \doh{}{\q}\Expec{\rhO'}{\int_{\q}\left(\frac{\rhO}{\rhO'}\right)^{\q} 
                                   \log\left(\frac{\rhO}{\rhO'}\right)\dif{\q}}
                                   \tag{Lebniz's rule} \\
                                   &= \q \doh{}{\q}\Expec{\rhO'}{\left(\frac{\rhO}{\rhO'}\right)^{\q}}
                                   = \q \doh{E(\q)}{\q}
                                   \tag{From \eqr{eqn:frenyi_divergence}}
    \end{align*}
    Moreover,
    \begin{align*}
        \Expec{\rhO'}{\norm{\graD{g}}^2} = \Expec{\rhO'}{\norm{\graD{
        \left(\frac{\rhO}{\rhO'}\right)^\frac{\q}{2}}}^2}
        = \frac{\q^2}{4} I(\q)
        \tag{From \eqr{eqn:grenyi_divergence}}
    \end{align*}
    Substituting \eqr{eqn:lsi_standard} with the above equalities give
    \begin{align*}
            &\Ent{\rhO'}{g^2} \leq \frac{2}{\alp} \Expec{\rhO'}{\norm{\graD{g}}^2} \\
        \iff&\q\doh{E(\q)}{\q} - E(\q) \log E(\q)
            \leq \frac{\q^2}{2\alp} I(\q) \\
        \iff&\q\doh{\log E(\q)}{\q} - \log E(\q) 
            \leq \frac{\q^2}{2\alp} \frac{I(\q)}{E(\q)} \\
        \iff&\q\doh{}{\q}\left((\q-1) R(\q)\right) - (\q - 1)R(\q)
            \leq \frac{\q^2}{2\alp} \frac{I(\q)}{E(\q)}
            \tag{From \eqr{eqn:renyi_divergence}} \\
	\iff& R(\q) + \q(\q-1)\doh{R(\q)}{\q}
            \leq \frac{\q^2}{2\alp} \frac{I(\q)}{E(\q)}
    \end{align*}
\end{proof}

\begin{reptheorem}{thm:linearRDP}
	Let $\loss{\x}{\ptheta}$ be a loss function on $\thetaspace$, with a finite total gradient sensitivity $\sen{\g}$, then the Langevin diffusion under loss $\ell(\theta;\x)$ and noise variance $\sig^2$ for time $T$ satisfies $(\alpha,\eps)$-RDP for $\eps=\frac{\alpha S_g^2 T}{4\sig^2\size^2}$.
\end{reptheorem}
\begin{proof}
    Setting $\gamma=1$ in Lemma~\ref{lem:marginalrenyi} gives constant privacy loss rate. Integrating over $t$ suffices.
\end{proof}

\begin{theorem}[RDP for Langevin Diffusion under $\alp$-LSI]
    \label{thm:RDboundCD}
    For a given dataset $\database \in \Domain$ and any $t>0$, let $\{\thet_t\}_{t\geq 0}$ be the Langevin diffusion on $\database$ for loss function ${\smaloss{\x}{\ptheta}}$ and variance~$\sig^2$.  If the distribution of $\thet_{t}$ satisfies $\alp$-LSI, for any~$\database$ and any $0\leq t\leq T$, the algorithm corresponding to the Langevin diffusion satisfies $(\q,\eps)$-RDP for
    \begin{equation} 
        \eps = \frac{\q S_g^2}{2 \alp n^2 \sig^4}(1-e^{-\sig^2\alp T})
    \end{equation}
    where $\sen{\g}$ is the finite sensitivity of total gradient ${\g(\ptheta; \D) = \sum_{\x \in \D} \graD{\loss{\x}{\ptheta}}}$.
\end{theorem}

\begin{proof}
	Let $a_1=2(1-\gamma)\sig^2\alp$, ${a_2=\frac{1}{\gamma}\frac{S_g^2}{4n^2\sig^2}}$, $y=log(\q-1)$, and ${u(t,y)=\frac{R(\q,t)}{\q}-\frac{a_2}{a_1}}$.  We re-write \eqr{eqn:EvolvePDE} as the following form of transport with decay PDE
	\begin{equation*}
	\frac{\partial u}{\partial t}+a_1 u+a_1\frac{\partial u}{\partial y}\leq 0,
	\end{equation*}
	with initial condition $u(0,y)=-\frac{a_2}{a_1}$. By introducing variables $\tau=t$, and $z=t-\frac{1}{a_1} y$ and writing $v(\tau,z)=u(t,y)$, we get $\frac{\partial v}{\partial \tau}+a_1 v\leq0$, with initial condition ${v(0,z) = u(0,-a_1 z)}$.  For every $z$, this means that the decay of $v$ is proportional to its present value. The solution for this problem is ${v(\tau,z) \leq v(0,z)e^{-a_1 \tau}}$.  By bringing back the original variables, we have
	\begin{equation*}
	u(t,y)\leq u(0,y-a_1 t)e^{-a_1 t}.
	\end{equation*}
	
	Therefore,
	\begin{align*}
	R(\q,t)&\leq \frac{a_2}{a_1}(1-e^{-a_1 t})\\
    &=\frac{\q S_g^2}{8\gamma(1-\gamma) \alp n^2 \sig^4}(1-e^{-\sig^2\alp T})\\
    &=\frac{\q S_g^2}{2 \alp n^2 \sig^4}(1-e^{-\sig^2\alp T})\quad\text{set }\gamma=\frac{1}{2}.
	\end{align*}
\end{proof}
