# Supplementary material for: Differential Privacy Dynamics of Langevin Diffusion and Noisy Gradient Descent
Source: arXiv:2102.05855 source file (2022-09-09)
Supplement: Supplementary file 6 [file smoothness.tex]

\section{Relaxing smoothness in Discretization}

Firstly, I derive a analogy lemma of Lemma~\ref{lem:new_delayed_loss_diff} which does not require smoothness of loss function.

\begin{lemma}
    \label{lem:nonsmooth_delayed_loss_diff}
    Let $\D, \D' \in \Domain$ be neighboring datasets of size $\size$. Let loss function  $\loss{\x}{\ptheta}$ be $\smh$-smooth, and sum of loss gradients $g(\ptheta;\D)=\sum_{\x_i\in\D}\nabla\ell(\ptheta;\x_i)$ has finite sensitivity $S_g$.
     For any $\tnoise^2$ and $\step$, given a sample $\thet_t \in \thetaspace$ at any time $t\geq0$, let r.v.'s $\thet_{\step\kk}, \thet_{\step\kk}', \thet_t, \thet_t'$ satisfy
    \begin{align}
        \label{eqn:new_delayed_update}
        \thet_{\step\kk} - (t-\step\kk) \graD{\Loss_\D(\thet_{\step\kk})} + \sqrt{2t\tnoise^2}\Z = \thet_t, \\
        \thet_{\step\kk}' - (t-\step\kk) \graD{\Loss_{\D'}(\thet_{\step\kk}')} + \sqrt{2t\tnoise^2}\Z' = \thet_t',
    \end{align}
    where $\Z, \Z' \sim \Gaus{0}{\Id}$, and $\kk$ is an integer s.t. ${\step\kk \leq t \leq \step(\kk+1)}$. Then, given $\ptheta_t$ was observed at time $t$, i.e. ${\thet_t = \thet_t' = \ptheta_t}$,
    \begin{align}
        \label{eqn:newdiscrete_error}
        \Big\Vert\Expec{}{\graD{\Loss_{\D}(\thet_{\step\kk})}\vert\ptheta_t} - &\Expec{}{\graD{\Loss_{\D'}(\thet_{\step\kk}')}\vert\ptheta_t}\Big\Vert_2^2 \leq \frac{S_g^2}{n^2(1-\step\be)^2}.
    \end{align}
\end{lemma}
